# Supplementary material for: Variations of the Hartree-Fock fractional-spin error for one electron
Source: arXiv:2105.07506 ancillary file (2021-06-30)
Supplement: Supplementary file 1 [file supplementary_material.pdf]

# Supplementary Material for "Variations of the Hartree–Fock fractional-spin error for one electron"

Hugh G. A. Burton,[1, a)] Clotilde Marut,[2] Timothy J. Daas,[3] Paola Gori-Giorgi,[3] and Pierre-François Loos[2, b)]
[1)]*Physical and Theoretical Chemical Laboratory, Department of Chemistry, University of Oxford, Oxford, OX1 3QZ, U.K.*
[2)]*Laboratoire de Chimie et Physique Quantiques, Université de Toulouse, CNRS, UPS, France*
[3)]*Department of Chemistry and Pharmaceutical Sciences, Amsterdam Institute of Molecular and Life Sciences (AIMMS), Faculty of Science, Vrije Universiteit, De Boelelaan 1083, 1081HV Amsterdam, The Netherlands*

In this supporting information, we compute high-accuracy fractional-spin energies for the restricted and unrestricted ensembles in the H atom (Fig. S1) alongside the associated density-driven errors. A large even-tempered basis set is employed for the H atom,[1] and the results can are considered to be converged with respect to the basis set size. These calculations are performed numerically using Mathematica 12.0.[2] The same basis set was employed to compute the change in the UHF radial probability density for different $w$ values (Fig. S2), as well as the radial spin-density probability for different $w$ values (Fig. S3).

We also compute accurate RHF and UHF energies for the fractional-spin $H_2^+$ cationic molecule (Fig. S4). These ensemble HF calculations[3,4] employ Dunning's cc-pVQZ basis set,[5] and are evaluated self-consistently using `QuAcK`,[6] an electronic structure program for emerging methods developed by one of the authors (PFL) and freely available on `github`.

All results gathered in this supporting information show the same phenomenology as the minimal basis results presented in the main text.

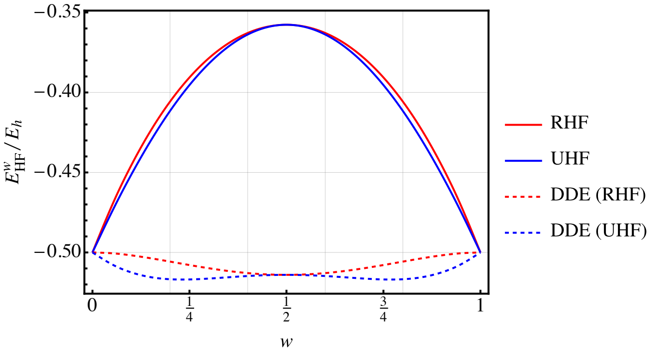


FIG. S1. Restricted (solid red) and unrestricted (solid blue) ensemble energies for the fractional-spin H atom at the Hartree–Fock level. The RHF and UHF density-driven errors (DDE) are also represented. These have been obtained using a large even-tempered basis set[1] and can be considered as converged with respect to the basis set.

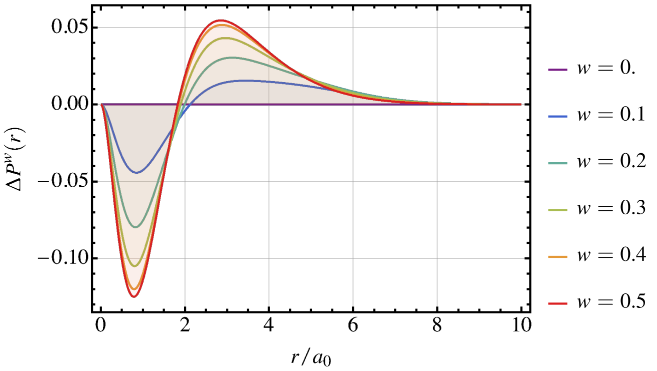


FIG. S2. Difference between unrestricted and exact radial probability densities for various weights $w$. These have been obtained using a large even-tempered basis set[1] and can be considered as converged with respect to the basis set.

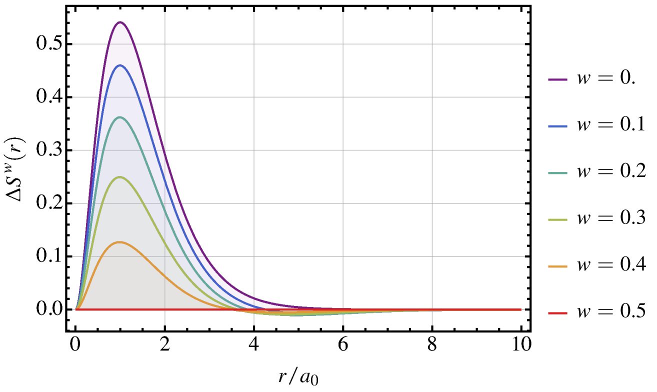


FIG. S3. Radial probability spin density of the unrestricted ground-state fractional-spin ensemble in the H atom for various $w$. These have been obtained using a large even-tempered basis set[1] and can be considered as converged with respect to the basis set.

[1]M. W. Schmidt and K. Ruedenberg, J. Chem. Phys. **71**, 3951 (1979).
[2]Wolfram Research, Inc., "Mathematica, Version 12.0," Champaign, IL, 2019.
[3]P.-F. Loos and E. Fromager, J. Chem. Phys. **152**, 214101 (2020).
[4]C. Marut, B. Senjean, E. Fromager, and P.-F. Loos, Faraday Discuss. **224**, 402 (2020).
[5]T. H. Dunning, J. Chem. Phys. **90**, 1007 (1989).
[6]P. F. Loos, "QuAcK: a software for emerging quantum electronic structure methods," (2019), https://github.com/pfloos/QuAcK.

[a)]Electronic mail: hugh.burton@chem.ox.ac.uk
[b)]Electronic mail: loos@irsamc.ups-tlse.fr

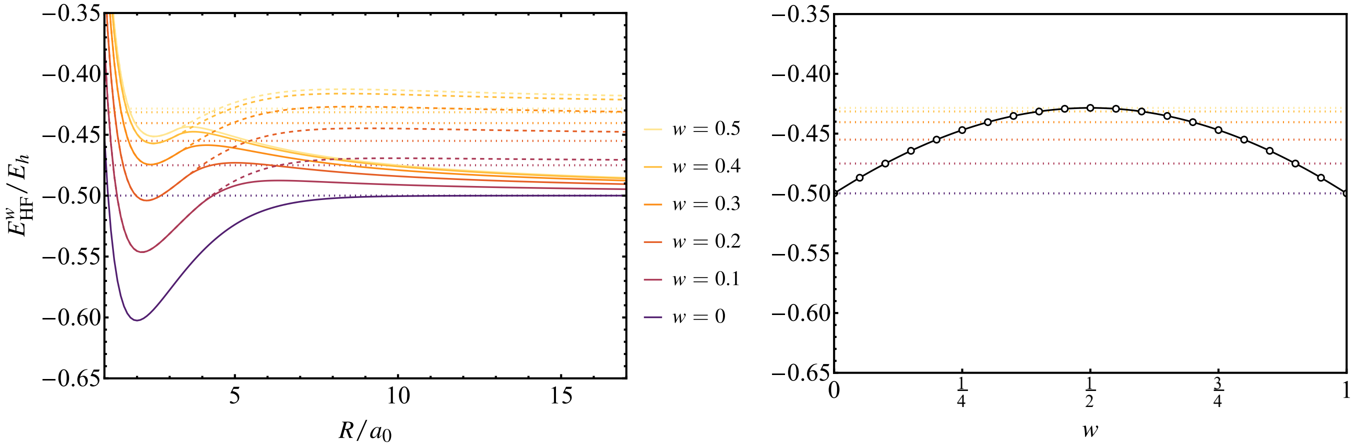


FIG. S4. Left: UHF (solid) and RHF (dashed) energies of $H_2{}^+$ as a function of the internuclear distance $R$ for various weights $w$. Right: RHF energies of $H_2{}^+$ in the dissociation limit as a function of the weight $w$. These have been obtained using Dunning's cc-pVQZ basis set.[5]
